# Supplementary material for: Certainty-Equivalence Model Predictive Control: Stability, Performance, and Beyond
Source: arXiv:2412.10625 source file (2026-02-03)
Supplement: Supplementary file 1 [file Lemma4_complex.tex]

\begin{proof}
	The proof employs induction. For $k = 0$, $\xi^{\star}_k(x';\para) = x'$, $\xi^{\star}_k(x'';\para) = x''$, and $\Gamma_{k} = 1$. Thus, \eqref{eq:lm4_open_loop_state_perturbation_bound} holds as an equality for $k = 0$. Assume that \eqref{eq:lm4_open_loop_state_perturbation_bound} holds for $k = k_0$ with $k_0 \in \bI_{0:N-1}$, i.e.,
	\begin{multline}
		\label{eq:B2_induction_assumption}
		\|\xi^\star_{k_0}(x';\para) - \xi^\star_{k_0}(x'';\para)\| \leq \\
		\left((\blfx)^{k_0} + \blfu\edsc\sum^{k_0-1}_{i=0}(\blfx)^i\edsr^{k_0-i}\right)\|x' - x''\|.
	\end{multline}
	Then, for $k = k_0 + 1$, it follows that
	\begin{align}
		& \|\xi^\star_{k_0+1}(x';\para) - \xi^\star_{k_0+1}(x'';\para)\| \notag \\
		= &\; \|f(\xi^\star_{k_0}(x';\para),u^\star_{k_0}(x';\para);\para) \sminus f(\xi^\star_{k_0}(x'';\para),u^\star_{k_0}(x'';\para);\para)\| \notag \\
		& \hspace*{-2.5ex} \overset{\eqref{eq:lipschitz_dynamics}}{\leq} \blfx\|\xi^\star_{k_0}(x';\para) - \xi^\star_{k_0}(x'';\para)\| + \notag \\
		& \hspace*{20ex} \blfu\|u^\star_{k_0}(x';\para) - u^\star_{k_0}(x'';\para)\| \notag \\
		& \hspace*{-1.5ex} \overset{\eqref{eq:subsec_eds:state_sensitivity_input},\eqref{eq:B2_induction_assumption}}{\leq} \left((\blfx)^{k_0+1} + \blfu\edsc\sum^{k_0-1}_{i=0}(\blfx)^{i+1}\edsr^{k_0-i} + \right. \notag \\
		& \hspace*{32ex} \blfu\edsc\edsr^{k_0}\Bigg)\|x' - x''\| \notag \\
		= & \left((\blfx)^{k_0+1} + \blfu\edsc\sum^{k_0}_{i=0}(\blfx)^{i}\edsr^{k_0+1-i} \right)\|x' - x''\|, \notag 
	\end{align}
	which completes the induction relation. A slight modified version of \eqref{eq:lm4_open_loop_state_perturbation_bound} that will be used later is
	\begin{equation}
		\label{eq:B2_final_conclusion}
		\|\xi^\star_{k}(\xp{\hpara};\hpara) - \xi^\star_{k}(\xp{\para};\hpara)\| \leq \Gamma_{k}\|\xp{\hpara} - \xp{\para}\|.
	\end{equation}
\end{proof}
