# Supplementary material for: Certainty-Equivalence Model Predictive Control: Stability, Performance, and Beyond
Source: arXiv:2412.10625 source file (2026-02-03)
Supplement: Supplementary file 2 [file Lemma6_complex.tex]

\begin{proof}
	For notational convenience, we define
	\begin{subequations}
		\label{eq:C2_definition}
		\begin{align}
			\label{eq:C2_def_state_dif}
			& \hspace*{-2ex} \Delta \xi^\star_{k}(x) := \xi^\star_{k}(x;\para) - \xi^\star_{k}(x;\hpara), \;\forall k \in \bI_{0:N}, \\
			\label{eq:C2_def_input_dif}
			& \hspace*{-2ex} \Delta u^\star_{k}(x) :=  u^\star_{k}(x;\para) - u^\star_{k}(x;\hpara) ,\;\forall k \in \bI_{0:N-1}, \\
			\label{eq:C2_def_pair}
			& \hspace*{-2ex} \Delta^\star_{f,k}(x;\hpara) := \Delta_f(\xi^\star_{k}(x;\hpara), u^\star_{k}(x;\hpara); \para),\;\forall k \in \bI_{0:N-1}.
		\end{align}
	\end{subequations}
	First, we establish the recursive relation between $\difxi{k+1}$ and $\difxi{k}$ as follows.
	\begin{align}
		\label{eq:C2_recursive_relation}
		& \;\difxi{k+1} \notag \\ 
		= & \;\|f(\xi^{\star}_k(x;\para), u^{\star}_k(x;\para); \para) \sminus f(\xi^{\star}_k(x;\hpara), u^{\star}_k(x;\hpara); \hpara)\| \notag \\
		\leq &\; \|f(\xi^{\star}_k(x;\para), u^{\star}_k(x;\para); \para) \sminus f(\xi^{\star}_k(x;\hpara), u^{\star}_k(x;\hpara); \para)\| + \notag \\
		&\; \hspace*{35ex} \dpairf{k} \notag \\
		& \hspace*{-2ex} \overset{\eqref{eq:lipschitz_dynamics}}{\leq}  \; L_{f,x}\difxi{k} + L_{f,u}\difu{k} + \dpairf{k},
	\end{align}
	where the second inequality is due to triangle inequality. Next, the main result \eqref{eq:open_loop_parameter_perturbation_bound} is proven by induction. For $k=0$, $C_{\Delta u,0}(\mpara;x) = 0$, $\sum^{-1}_{i=0}[\cdot] = 0$, and $\xi^\star_{0}(x;\para) - \xi^\star_{0}(x;\hpara) = x - x = 0$. Thus, \eqref{eq:open_loop_parameter_perturbation_bound} holds trivially with both sides equal to $0$. Assume that \eqref{eq:open_loop_parameter_perturbation_bound} holds for $k = k_0$, i.e.,
	\begin{multline}
		\label{eq:C2_induction_assumption}
		\difxi{k_0} \leq L_{f,u}\sum^{k_0-1}_{i=0}L^{k_0-1-i}_{f,x}\sueds{i}(\mpara;\|x\|) + \\ \sum^{k_0-1}_{i=0}L^{k_0-1-i}_{f,x}\|\Delta f(\xi^\star_{i}(x;\hpara),u^\star_{i}(x;\hpara);\para)\|.
	\end{multline}
	Then, for $k = k_0 + 1$, it holds that
	\begin{align}
		% \label{eq:C2_induction_prove}
		& \hspace*{4ex} \difxi{k_0+1} \notag \\
		& \overset{\eqref{eq:C2_recursive_relation}}{\leq} L_{f,x}\difxi{k_0} + L_{f,u}\difu{k_0} + \dpairf{k_0} \notag \\
		&  \overset{\eqref{eq:C2_induction_assumption}}{\leq} L_{f,u}\sum^{k_0-1}_{i=0}L^{k_0-i}_{f,x}\sueds{i}(\mpara;\|x\|) \splus \sum^{k_0-1}_{i=0}L^{k_0-i}_{f,x}\dpairf{i} \notag \\
		& \hspace*{5ex} + L_{f,u}\difu{k_0} + \dpairf{k_0} \notag \\ 
		&  \overset{\eqref{eq:subsec_para_perturbation:refined_eds}}{\leq} L_{f,u}\sum^{k_0-1}_{i=0}L^{k_0-i}_{f,x}\sueds{i}(\mpara;\|x\|) \splus \sum^{k_0-1}_{i=0}L^{k_0-i}_{f,x}\dpairf{i} \notag \\
		& \hspace*{5ex} + L_{f,u}\sueds{k_0}(\mpara; \|x\|) + \dpairf{k_0} \notag \\
		& \hspace*{1ex} \leq L_{f,u}\sum^{k_0}_{i=0}L^{k_0-i}_{f,x}\sueds{i}(\mpara;\|x\|) + \sum^{k_0}_{i=0}L^{k_0-i}_{f,x}\dpairf{i}, \notag
	\end{align}
	which completes the induction relation.
\end{proof}
