# Supplementary material for: Certainty-Equivalence Model Predictive Control: Stability, Performance, and Beyond
Source: arXiv:2412.10625 source file (2026-02-03)
Supplement: Supplementary file 3 [file Prop2_complex.tex]

\begin{proof}
	The left inequality of \eqref{eq:nominal_bound} is due to
	\begin{equation*}
		\cost^\star(x) \leq \cost(x, \mu_{N,\hpara}(x)) \leq V_{N}(x;\para),
	\end{equation*}
	and the right inequality is a direct consequence of \eqref{eq:sec_prob:mpc_linear_bound}. To prove \eqref{eq:nominal_decreasing}, we employ the \textit{case distinction} method in \cite{kohler2023stability}. More specifically, the final cost evaluated at stage $N$, i.e., $\cost^\star(\xi^\star_N(x;\hpara))$, is used as the distinction variable. First, assume that
	\begin{equation}
		\label{eq:B1_case1_assumption}
		\cost^\star(\xi^\star_N(x;\hpara)) \leq \frac{(1 + \umpc)\mpc_{N}}{(N -1)\lyacf + N + \umpc}\cost^\star(x).
	\end{equation}
	By definition, it holds that
	\begin{multline}
		\label{eq:B1_firstcase_ground}
		V_N(\xp{\hpara};\hpara) =  \cost^\star(\xi^\star_N(\xp{\hpara};\hpara)) + \\ \sum^{N-1}_{k=0}\cost(\xi^\star_k(\xp{\hpara};\hpara), u^\star_k(\xp{\hpara};\hpara)).
	\end{multline}
	Due to the optimality of $\mathbf{u}^\star_N(\xp{\hpara};\hpara)$, \eqref{eq:B1_firstcase_ground} implies that
	\begin{align}
		\label{eq:B1_firstcase_main_derivation}
		& V_N(\xp{\hpara};\hpara) \notag \\
		\leq & \; \cost^\star(f(\xi^\star_N(x;\hpara), \uclf;\hpara) + \notag \\
		& \;\cost(\xi^\star_N(x;\hpara), \uclf) + \sum^{N-1}_{k=1}\cost(\xi^\star_{k}(x;\hpara), u^\star_{k}(x;\hpara)) \notag \\
		\leq &  \; \cost^\star(f(\xi^\star_N(x;\hpara), \uclf;\hpara) + \cost(\xi^\star_N(x;\hpara), \uclf) + \notag \\
		& \;V_N(x;\hpara) - \cost(x, \mu_{N,\hpara}(x)) - \cost^\star(\xi^\star_N(x;\hpara)) \notag \\
		\overset{\eqref{eq:sec_prob:relaxed_clf}}{\leq} & \;\lyacf \cost^\star(\xi^\star_N(x;\hpara)) + V_N(x;\hpara) - \cost(x, \mu_{N,\hpara}(x)),
	\end{align}
	where the second inequality is due to the definition of $V_N(x;\hpara)$. \eqref{eq:B1_firstcase_main_derivation} is equivalent to
	\begin{align}
		\label{eq:B1_firstcase_final}
		& \;V_N(\xp{\hpara};\hpara) - V_N(x;\hpara) \notag \\ 
		\leq  & \; - \cost(x, \mu_{N,\hpara}(x)) + \lyacf \cost^\star(\xi^\star_N(x;\hpara)) \notag \\
		\overset{\eqref{eq:B1_case1_assumption}}{\leq} & \; - \cost(x, \mu_{N,\hpara}(x)) + \frac{(1 + \umpc)\mpc_{N}\lyacf}{(N -1)\lyacf + N + \umpc}\cost^\star(x) \notag \\
		\leq &\; -(1 - \epsilon_N)\cost(x, \mu_{N,\hpara}(x)),
	\end{align}
	where $\epsilon_N := \frac{(1 + \umpc)\mpc_{N}\lyacf}{(N -1)\lyacf + N + \umpc}$. On the other hand, assume that
	\begin{equation}
		\label{eq:B1_case2_assumption}
		\cost^\star(\xi^\star_N(x;\hpara)) \geq \frac{(1 + \umpc)\mpc_{N}}{(N -1)\lyacf + N + \umpc}\cost^\star(x).
	\end{equation}
	By definition, it holds that
	\begin{multline}
		\label{eq:B1_case2_ground}
		\sum^{N-1}_{k=0}\cost^\star(\xi^\star_k(x;\hpara)) \leq V_N(x;\hpara) - \cost^\star(\xi^\star_N(x;\hpara)) \\
		\overset{\eqref{eq:sec_prob:mpc_linear_bound},\eqref{eq:B1_case2_assumption}}{\leq} \left(1 + \mpc_{N} - \frac{(1 + \umpc)\mpc_{N}}{(N -1)\lyacf + N + \umpc}\right)\cost^\star(x).
	\end{multline}
	Subtracting $\cost^\star(x)$ on both sides of \eqref{eq:B1_case2_ground} yields
	\begin{equation}
		\label{eq:B1_case2_turnpoint}
		\sum^{N-1}_{k=1}\cost^\star(\xi^\star_k(x;\hpara)) \leq \frac{\mpc_{N}(1 + \lyacf)(N -1)}{(N-1)\lyacf + N + \umpc}\cost^\star(x),
	\end{equation} 
	which indicates that $\exists k^\ast \in \bI_{1:N-1}$ such that
	\begin{equation}
		\label{eq:B1_case2_turnpoint_base}
		\cost^\star(\xi^\star_{k^\ast}(x;\hpara)) \leq \frac{\mpc_{N}(1 + \lyacf)}{(N-1)\lyacf + N + \umpc}\cost^\star(x).
	\end{equation}
	Then, it holds that
	\begin{align}
		& \;V_{N}(\xp{\hpara}) + \cost(x, \mu_{N,\hpara}(x)) \notag \\
		\leq &\; J_{k^\ast}(x, \mathbf{u}^\ast_N(x;\hpara)) + V_{N-k^\ast+1}(\cost^\star(\xi^\star_{k^\ast}(x;\hpara))) \notag \\
		\overset{\eqref{eq:sec_prob:mpc_linear_bound}}{\leq} &\; V_N(x;\hpara) - \cost^\star(\xi^\star_N(x;\hpara)) + (1 + \umpc) \cost^\star(\xi^\star_{k^\ast}(x;\hpara)) \notag \\
		&\hspace*{-2ex} \overset{\eqref{eq:B1_case2_assumption},\eqref{eq:B1_case2_turnpoint_base}}{\leq} \; V_N(x;\hpara) + \frac{(1 + \umpc)\mpc_{N}\lyacf}{(N -1)\lyacf + N + \umpc}\cost^\star(x),
	\end{align}
	which again implies that
	\begin{equation}
		\label{eq:B1_case2_conclusion}
		V_N(\xp{\hpara};\hpara) - V_N(x;\hpara) \leq -(1 - \epsilon_N)\cost(x, \mu_{N,\hpara}(x)).
	\end{equation}
	Therefore, in both cases the desired property \eqref{eq:B1_case2_conclusion} (cf. \eqref{eq:nominal_decreasing}) is established. Besides, it holds that
	\begin{align}
		\label{eq:B3_energy_decreasing}
		& \;V_N(\xp{\hpara};\hpara) \notag \\
		\overset{\eqref{eq:B1_case2_conclusion}}{\leq} & \;V_N(x;\hpara) - (1 - \epsilon_N)\cost(x, \mu_{N,\hpara}(x))\notag  \\ 
		\overset{\eqref{eq:sec_prob:mpc_linear_bound}}{\leq} & \;(1 + \mpc_N)\cost^\star(x) - (1 - \epsilon_N)\cost(x, \mu_{N,\hpara}(x))\notag  \\ 
		\leq & \;(1 + \mpc_N)\cost(x, \mu_{N,\hpara}(x)) - (1 - \epsilon_N)\cost(x, \mu_{N,\hpara}(x))\notag  \\ 
		\leq & \;(\mpc_N + \epsilon_N)\cost(x, \mu_{N,\hpara}(x)),
	\end{align}
	which completes the proof.
\end{proof}
